# Supplementary material for: A new method to detect globular clusters with the S-PLUS survey
Source: arXiv:2111.14993 source file (2021-11-29)
Supplement: Supplementary file 1 [file appendix.tex]

\section{SED fitting}

\begin{figure*}
    \centering
    \includegraphics[width=\textwidth]{Figures/composed.png}
    \caption{Caption}
    \label{fig:my_label}
\end{figure*}
